# Supplementary material for: Unstable Optical Resonators & Fractal Light
Source: arXiv:physics/0612027 source file (2006-12-03)
Supplement: Supplementary file 1 [file appendix.tex]

\documentclass[10pt,a4,a4paper]{report}
\usepackage[dvips]{graphicx}
\usepackage{listings}

\begin{document}

\appendix

\chapter{Cavity Simulator Codes}
\lstset{basicstyle=\scriptsize,breaklines=true}
\lstinputlisting{cavity_sim.c}

\clearpage
\chapter{Video Fractal Codes}
\lstset{basicstyle=\scriptsize,breaklines=true}
\lstinputlisting{vf.c}

\end{document}
